# Supplementary material for: First-principles predicted low-energy structures of NaSc(BH4)4
Source: arXiv:1306.1968 source file (2014-03-29)
Supplement: Supplementary file 1 [file supplement_NaSc.pdf]

# Supplemental Material: First-principles predicted low-energy structures of $NaSc(BH_4)_4$

Huan Doan Tran,[1] Maximilian Amsler,[1] Silvana Botti,[2] Miguel A. L. Marques,[2] and Stefan Goedecker[1]
[1)] *Department of Physics, Universität Basel, Klingelbergstrasse 82, 4056 Basel, Switzerland*[a)]
[2)] *Université de Lyon, F-69000 Lyon, France and LPMCN, CNRS, UMR 5586, Université Lyon 1, F-69622 Villeurbanne, France*

(Dated: 10 March 2014)

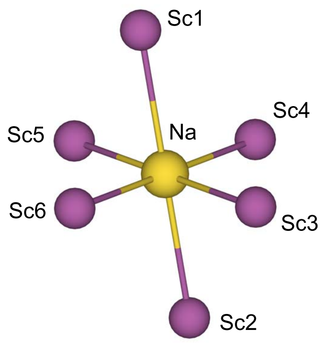


FIG. 1. (Color online) Six-fold coordinations of sodium in the *Cmcm* structure of $NaSc(BH_4)_2$.

TABLE III: Crystallographic information of the low-energy structures of $NaSc(BH_4)_4$ discovered in this work. For each structure, cell parameters are given while for each atom, Wyckoff possition and coordinates ($x$, $y$, and $z$) are given.

| $C222_1$ | $a$ (Å) | $b$ (Å) | $c$ (Å) | $\alpha$ (°) | $\beta$ (°) | $\gamma$ (°) |
|---|---|---|---|---|---|---|
| (20) | 8.318 | 11.827 | 9.117 | 90 | 90 | 90 |

| Atom | $x$ | $y$ | $z$ |
|---|---|---|---|
| Na (4a) | 0.073220 | 0.000000 | 0.000000 |
| Sc (4b) | 0.000000 | 0.345770 | 0.250000 |
| B (8c) | −0.499410 | 0.266140 | −0.456900 |
| B (8c) | 0.271250 | 0.041520 | −0.250310 |
| H (8c) | −0.493270 | 0.321510 | 0.432330 |
| H (8c) | 0.393510 | 0.296020 | −0.370490 |
| H (8c) | 0.128970 | 0.230420 | 0.387930 |
| H (8c) | −0.350120 | 0.485680 | −0.257530 |
| H (8c) | 0.243230 | 0.142880 | −0.271030 |
| H (8c) | 0.370200 | 0.010580 | −0.342980 |
| H (8c) | 0.160750 | 0.466210 | 0.370300 |
| H (8c) | 0.473650 | 0.165920 | −0.486390 |

| $C2$ | $a$ (Å) | $b$ (Å) | $c$ (Å) | $\alpha$ (°) | $\beta$ (°) | $\gamma$ (°) |
|---|---|---|---|---|---|---|
| (5) | 8.850 | 12.963 | 6.228 | 90 | 134.53 | 90 |

| Atom | $x$ | $y$ | $z$ |
|---|---|---|---|
| Na (2b) | 0.00000 | 0.43954 | 0.50000 |
| Sc (2a) | 0.00000 | 0.18802 | 0.00000 |

to be continued ..

[a)] Present address of HDT: Institute of Materials Science, University of Connecticut, 97 North Eagleville Rd., Unit 3136, Storrs, CT 06269-3136, USA; email: huan.tran@uconn.edu

**TABLE III – continued from previous page**

| | | | |
|---|---|---|---|
| B (4c) | 0.23382 | 0.08404 | 0.04507 |
| B (4c) | 0.18585 | 0.29231 | 0.42176 |
| H (4c) | 0.35209 | 0.03029 | 0.05962 |
| H (4c) | −0.26106 | 0.07828 | −0.26968 |
| H (4c) | −0.00416 | 0.31724 | 0.22018 |
| H (4c) | −0.28831 | 0.34516 | 0.35493 |
| H (4c) | 0.04610 | 0.06084 | −0.17362 |
| H (4c) | −0.25610 | 0.17617 | −0.02184 |
| H (4c) | −0.25511 | 0.29766 | −0.30539 |
| H (4c) | −0.18755 | 0.20062 | −0.47815 |

| $Cc$ | $a$ (Å) | $b$ (Å) | $c$ (Å) | $\alpha$ (°) | $\beta$ (°) | $\gamma$ (°) |
|---|---|---|---|---|---|---|
| (9) | 9.048 | 8.740 | 12.808 | 90 | 85.86 | 90 |

| Atom | $x$ | $y$ | $z$ |
|---|---|---|---|
| Na (4a) | 0.09566 | 0.24312 | 0.06293 |
| Sc (4a) | −0.15256 | 0.02927 | −0.18598 |
| B (4a) | −0.17061 | 0.18849 | 0.41706 |
| B (4a) | 0.37950 | 0.26077 | 0.42046 |
| B (4a) | 0.13347 | 0.44301 | 0.22689 |
| B (4a) | −0.45200 | 0.49197 | 0.19139 |
| H (4a) | −0.17531 | 0.30362 | 0.46921 |
| H (4a) | 0.39306 | 0.15192 | 0.47694 |
| H (4a) | 0.49042 | 0.34537 | 0.41263 |
| H (4a) | −0.27812 | 0.10149 | 0.43530 |
| H (4a) | 0.44061 | 0.38858 | −0.06801 |
| H (4a) | −0.22573 | 0.15700 | −0.04769 |
| H (4a) | 0.01973 | 0.43390 | 0.18352 |
| H (4a) | −0.34562 | 0.49915 | 0.12901 |
| H (4a) | 0.19095 | 0.42936 | −0.28609 |
| H (4a) | −0.00691 | 0.13756 | −0.30674 |
| H (4a) | 0.35906 | 0.22129 | 0.33008 |
| H (4a) | −0.16775 | 0.21801 | 0.32253 |
| H (4a) | −0.05425 | 0.08013 | 0.17169 |
| H (4a) | 0.23002 | 0.34896 | 0.19578 |
| H (4a) | 0.08049 | 0.02337 | 0.28111 |
| H (4a) | 0.11177 | 0.42103 | 0.32210 |

| $P1$ | $a$ (Å) | $b$ (Å) | $c$ (Å) | $\alpha$ (°) | $\beta$ (°) | $\gamma$ (°) |
|---|---|---|---|---|---|---|
| (1) | 13.497 | 6.329 | 6.041 | 89.48 | 77.19 | 103.44 |

| Atom | $x$ | $y$ | $z$ |
|---|---|---|---|
| Na (1a) | −0.07392 | 0.46299 | −0.46295 |
| Na (1a) | 0.43822 | 0.21911 | −0.21922 |
| Sc (1a) | 0.18624 | −0.40687 | −0.09311 |
| Sc (1a) | −0.31759 | −0.15880 | −0.34121 |
| B (1a) | −0.42415 | 0.00583 | 0.49903 |
| B (1a) | −0.42416 | −0.43000 | −0.07491 |
| B (1a) | 0.07976 | −0.27311 | −0.28245 |
| B (1a) | 0.07976 | 0.35289 | 0.20269 |
| B (1a) | −0.21092 | −0.31876 | 0.39149 |
| B (1a) | −0.21094 | 0.10782 | −0.18053 |
| B (1a) | 0.29195 | 0.41391 | −0.33844 |
| B (1a) | 0.29196 | −0.12194 | 0.04648 |

to be continued ..

TABLE I. Lattice parameters from the DFT optimized *Cmcm* structure $NaSc(BH_4)_4$, given in Å. The space group of the structure was not changed by the optimization. Experimental data are taken from Černý *et al.*, J. Phys. Chem. C **114**, 1357 (2010).

| | PW91 | | PBE | | PBEsol | | LDA | | vdW-DF2 | | DFT-D2 | | DFT-TS | | Expr. |
|---|---|---|---|---|---|---|---|---|---|---|---|---|---|---|---|
| | DFT | Δ(%) | DFT | Δ(%) | DFT | Δ(%) | DFT | Δ(%) | DFT | Δ(%) | DFT | Δ(%) | DFT | Δ(%) | |
| $a$(Å) | 8.109 | −0.7 | 8.122 | −0.6 | 7.926 | −3.0 | 7.733 | −5.4 | 8.088 | −1.0 | 7.712 | −5.6 | 7.904 | −3.3 | 8.170 |
| $b$(Å) | 11.900 | 0.2 | 11.904 | 0.2 | 11.586 | −2.4 | 11.245 | −5.3 | 11.765 | −0.9 | 11.321 | −4.7 | 11.312 | −4.7 | 11.875 |
| $c$(Å) | 8.967 | −0.6 | 8.973 | −0.5 | 8.668 | −3.9 | 8.317 | −7.7 | 8.640 | −4.2 | 8.263 | −8.4 | 8.168 | −9.4 | 9.018 |
| $V$(Å$^3$) | 865.4 | −1.1 | 867.6 | −0.8 | 795.9 | −9.0 | 723.2 | −17.3 | 822.2 | −6.0 | 721.4 | −17.5 | 730.3 | −16.5 | 874.9 |

TABLE II. Na-Sc "bond" lengths obtained with PBE and vdW-DF2, given in Å, and the corresponding difference Δ from the experimental data, of the optimized *Cmcm* structure. Labels of these bonds are defined in Fig. 1.

| Bond | Expr. | PBE | | vdW-DF2 | |
|---|---|---|---|---|---|
| | | DFT | Δ (%) | DFT | Δ(%) |
| Na-Sc1 | 4.779 | 4.747 | −0.67 | 4.679 | −2.09 |
| Na-Sc2 | 4.779 | 4.747 | −0.67 | 4.679 | −2.09 |
| Na-Sc3 | 4.989 | 4.965 | −0.48 | 4.894 | −1.90 |
| Na-Sc4 | 4.989 | 4.965 | −0.48 | 4.894 | −1.90 |
| Na-Sc5 | 4.989 | 4.965 | −0.48 | 4.894 | −1.90 |
| Na-Sc6 | 4.989 | 4.965 | −0.48 | 4.894 | −1.90 |

**TABLE III – continued from previous page**

| | | | |
|---|---|---|---|
| H (1a) | −0.48003 | 0.09154 | 0.41744 |
| H (1a) | −0.48004 | 0.42841 | 0.06255 |
| H (1a) | 0.17275 | −0.22190 | −0.38536 |
| H (1a) | 0.17275 | 0.39466 | 0.21261 |
| H (1a) | 0.02539 | 0.22362 | 0.35438 |
| H (1a) | 0.02539 | −0.19823 | −0.37977 |
| H (1a) | −0.44979 | −0.25493 | −0.04904 |
| H (1a) | −0.44978 | −0.19486 | 0.49881 |
| H (1a) | 0.05585 | −0.46878 | 0.20314 |
| H (1a) | 0.05587 | −0.47535 | −0.25898 |
| H (1a) | 0.07400 | −0.20985 | −0.08801 |
| H (1a) | 0.07399 | 0.28387 | 0.01402 |
| H (1a) | −0.20992 | −0.36544 | −0.40846 |
| H (1a) | −0.20993 | 0.15552 | −0.38157 |
| H (1a) | 0.29985 | 0.39283 | −0.13861 |
| H (1a) | 0.29985 | −0.09298 | −0.16126 |
| H (1a) | −0.15517 | 0.24734 | −0.09856 |
| H (1a) | −0.15515 | −0.40252 | 0.25377 |
| H (1a) | 0.34647 | 0.02228 | 0.12595 |
| H (1a) | 0.34645 | 0.32420 | −0.47246 |
| H (1a) | −0.42568 | 0.04722 | −0.29929 |
| H (1a) | −0.42568 | −0.47289 | −0.27507 |
| H (1a) | −0.33129 | −0.39820 | −0.06584 |
| H (1a) | −0.33128 | 0.06690 | 0.39710 |
| H (1a) | −0.18476 | −0.06698 | −0.18237 |
| H (1a) | −0.18475 | −0.11779 | 0.36715 |
| H (1a) | 0.31379 | −0.29842 | 0.07285 |
| H (1a) | 0.31379 | −0.38777 | −0.38665 |
| H (1a) | −0.30375 | 0.07373 | −0.07775 |
| H (1a) | −0.30372 | −0.37748 | 0.38151 |
| H (1a) | 0.19829 | −0.14313 | 0.13602 |

to be continued ..

**TABLE III – continued from previous page**

| | | | | | | |
|---|---|---|---|---|---|---|
| H (1a) | | 0.19828 | | 0.34143 | | −0.33428 |
| $I222$ | $a$ (Å) | $b$ (Å) | $c$ (Å) | $\alpha$ (°) | $\beta$ (°) | $\gamma$ (°) |
| (23) | 12.332 | 6.355 | 6.353 | 90 | 90 | 90 |
| Atom | | $x$ | | $y$ | | $z$ |
| Na (2c) | | 0.00000 | | 0.00000 | | 0.50000 |
| Sc (2d) | | 0.00000 | | 0.50000 | | 0.00000 |
| B (8k) | | −0.39622 | | 0.21586 | | 0.28431 |
| H (8k) | | −0.34249 | | 0.32747 | | 0.17142 |
| H (8k) | | 0.49463 | | −0.25920 | | 0.28055 |
| H (8k) | | 0.36900 | | −0.23135 | | 0.47096 |
| H (8k) | | −0.38935 | | 0.02848 | | 0.23393 |

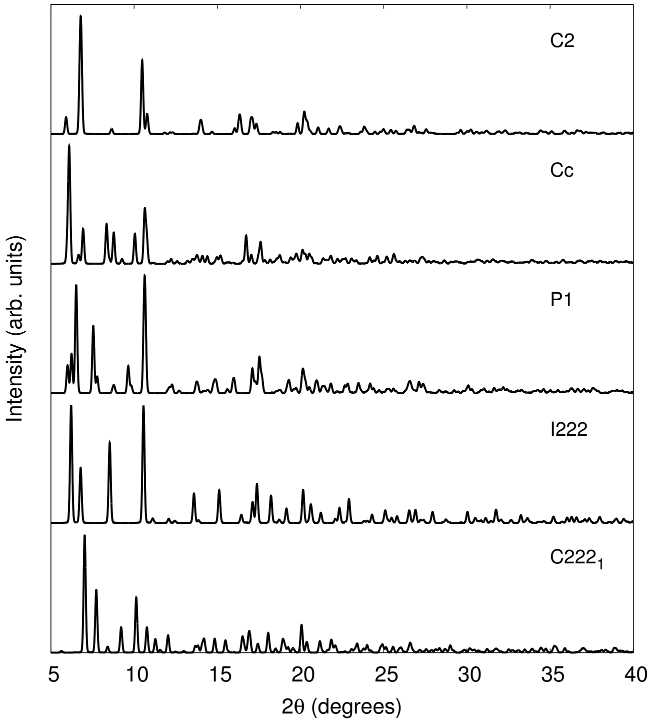


FIG. 2. Simulated powder x-ray diffraction patterns of the examined low-energy structures of $NaSc(BH_4)_4$.

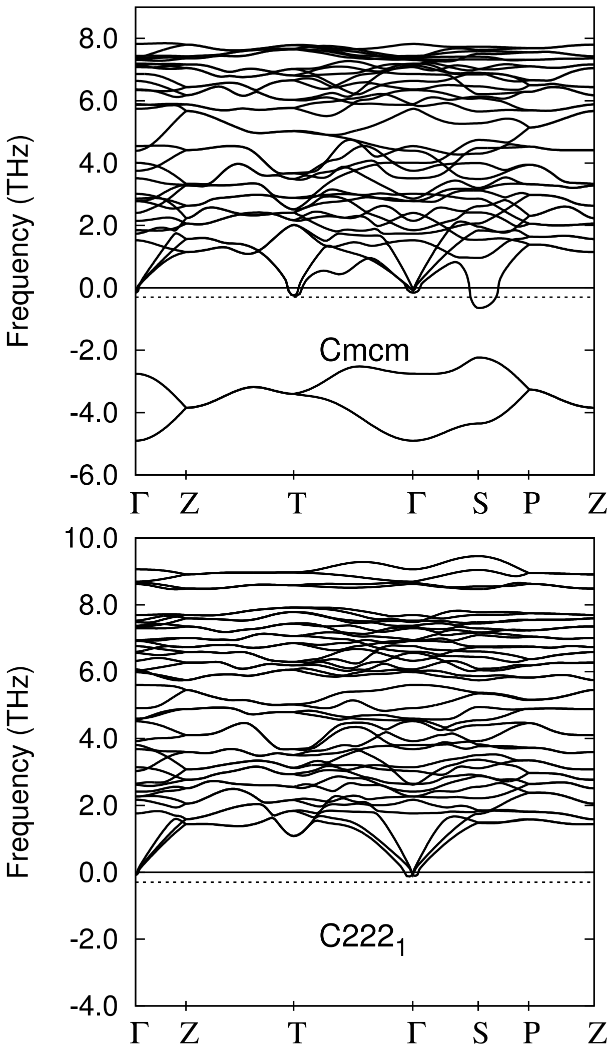


FIG. 3. Phonon band structures of the $Cmcm$ and $C222_1$ structures of $NaSc(BH_4)_4$. The van der Waals in these structures are calculated with vdW-DF2. Dotted lines indicate the lower bound corresponding to the errorbar of $\sim 0.3$ THz due to the numerically unresolved translational invariance in calculations of the XC energies.

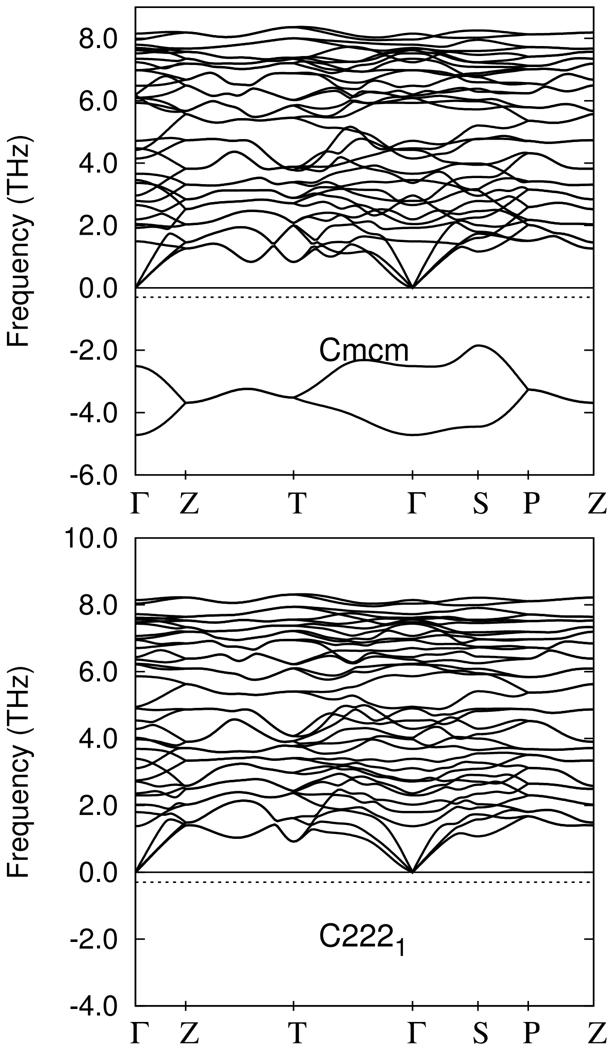


FIG. 4. Phonon band structures of the *Cmcm* and $C222_1$ structures of $NaSc(BH_4)_4$. LDA is used for the calculations leading to this result. Dotted lines indicate the lower bound corresponding to the errorbar of $\sim$ 0.3 THz due to the numerically unresolved translational invariance in calculations of the XC energies.

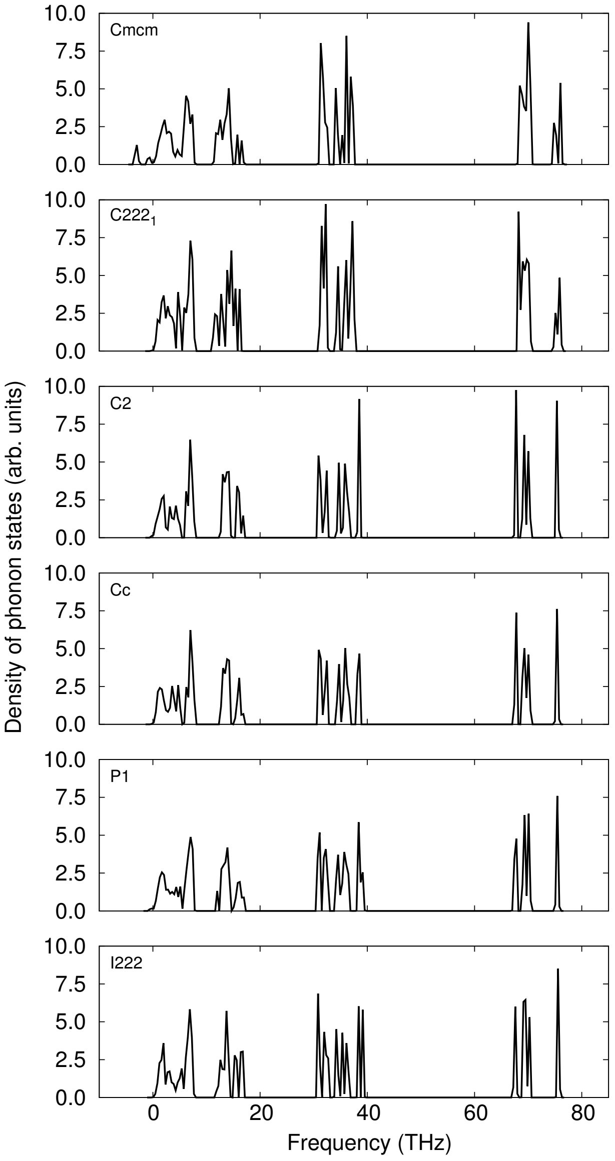


FIG. 5. Phonon densities of states of the low-energy structures discovered for $NaSc(BH_4)_4$.
